# Supplementary material for: Tuning the Spin Interaction in Non-planar Organic Diradicals Through Mechanical Manipulation
Source: arXiv:2402.08641 source file (2024-02-13)

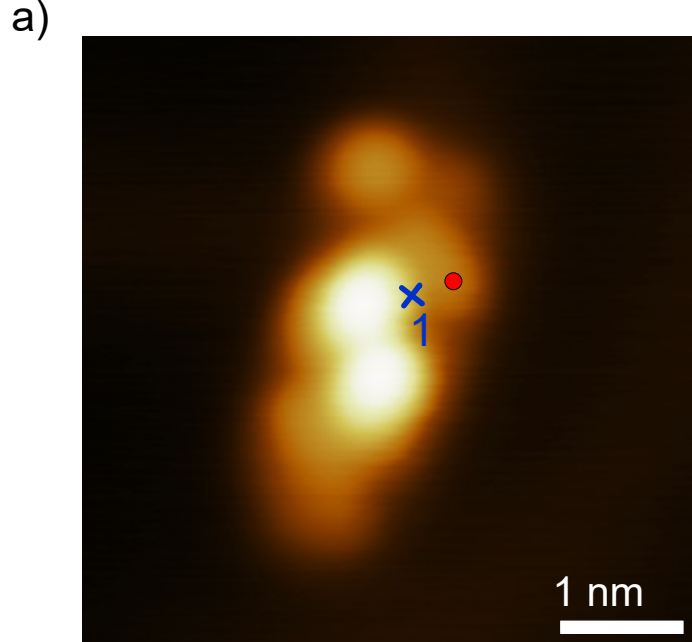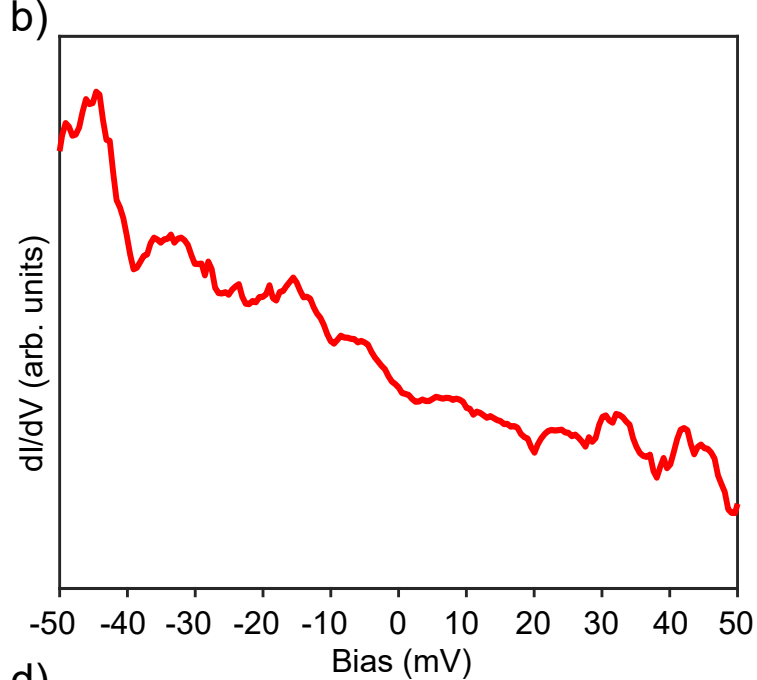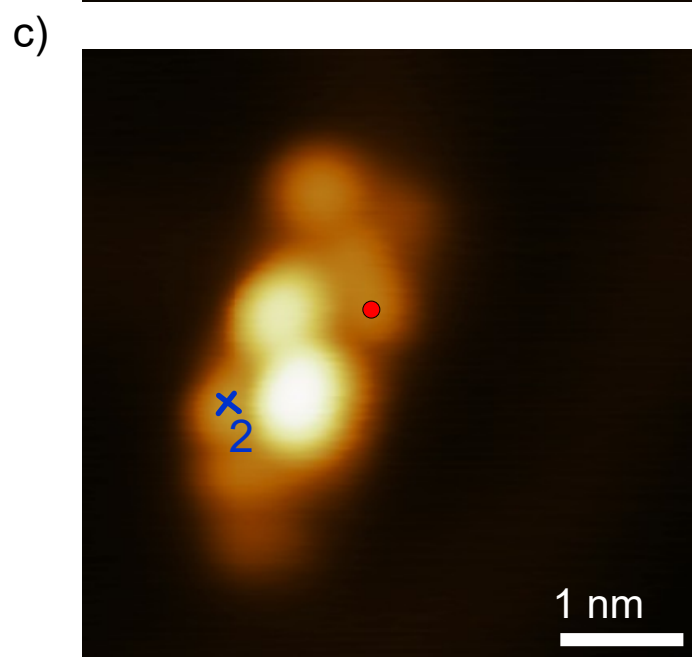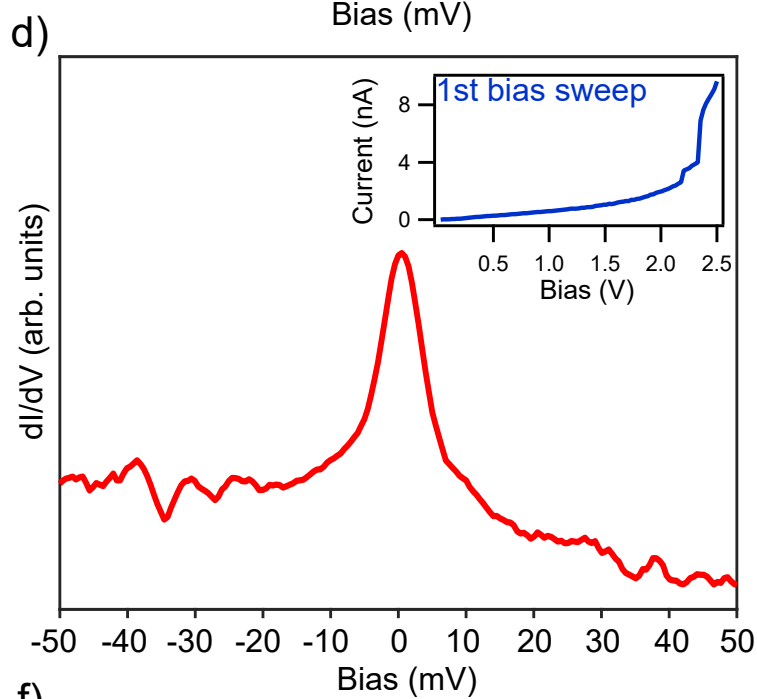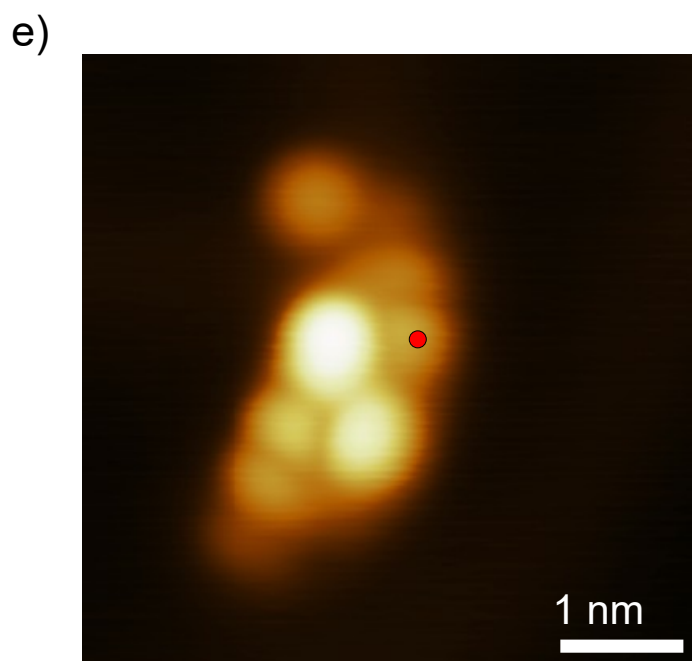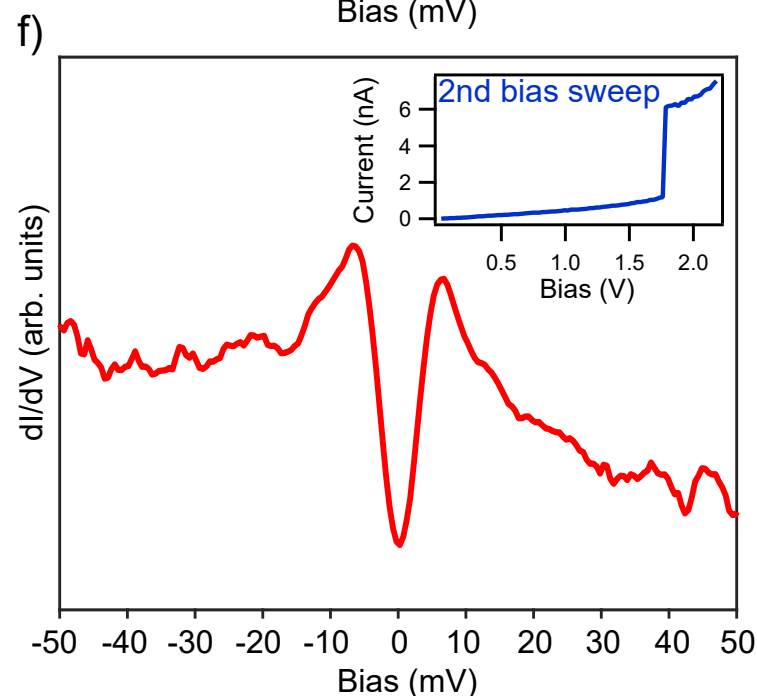

Supplement: Supplementary file 1 [file SI3_SMe2OS_bias_sweep.pdf]
