# Supplementary material for: Tuning the Spin Interaction in Non-planar Organic Diradicals Through Mechanical Manipulation
Source: arXiv:2402.08641 source file (2024-02-13)

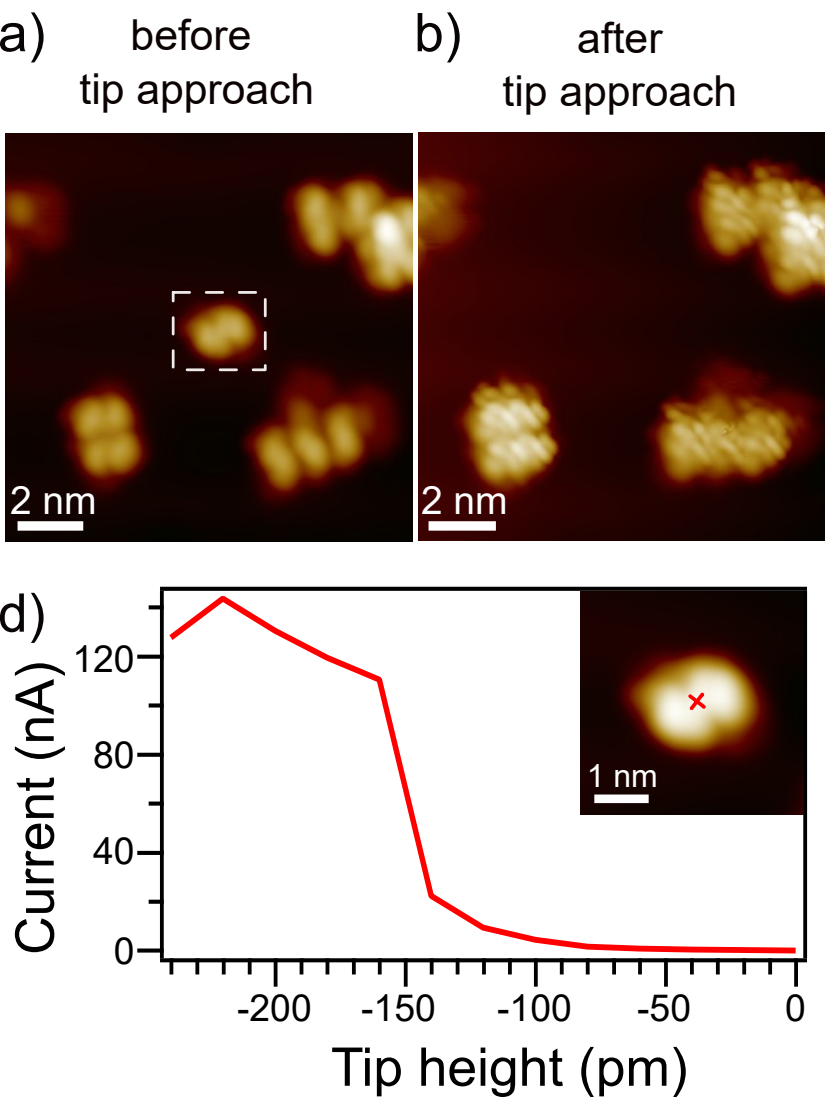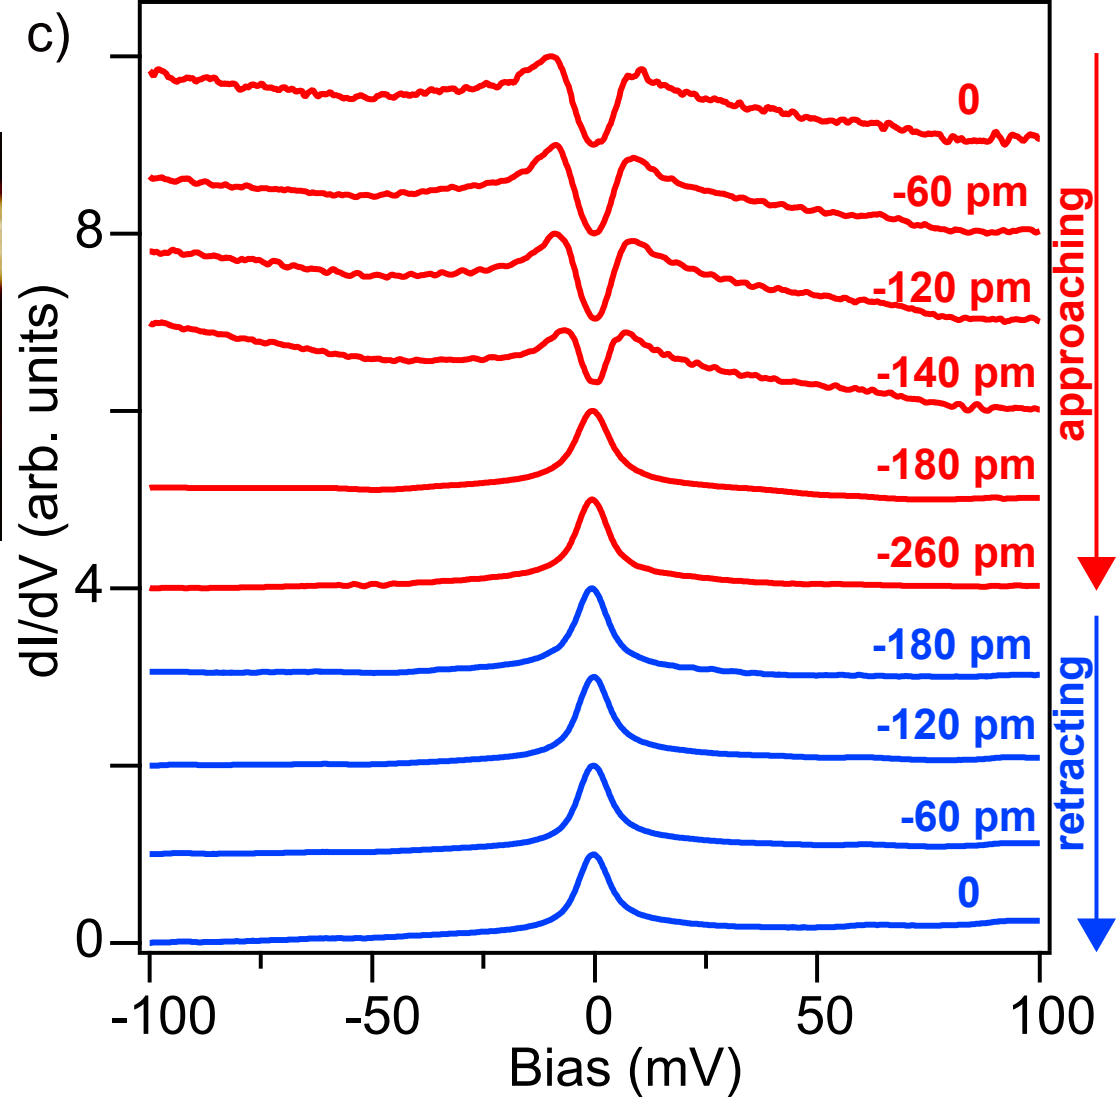

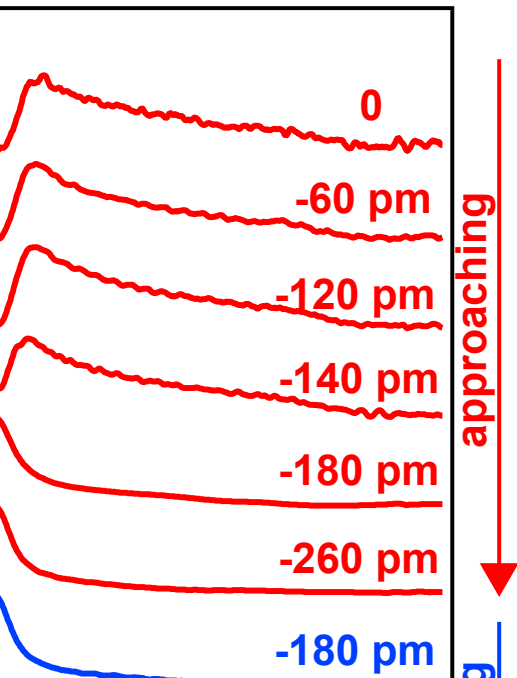

Supplement: Supplementary file 2 [file SI_2OS_manipulation.pdf]
